# Supplementary material for: LayerBuilder: Layer Decomposition for Interactive Image and Video Color Editing
Source: arXiv:1701.03754 ancillary file (2017-01-16)
Supplement: Supplementary file 1 [file supplemental-arxiv.pdf]

# LayerBuilder: Layer Decomposition for Interactive Image and Video Color Editing (Supplemental Materials)

### Recoloring Comparisons

Additional recoloring comparisons to RBF interpolation, manifold-preserving edit propagation, and palette-based RBF interpolation are shown in Figure 1.

### Photoshop Comparison

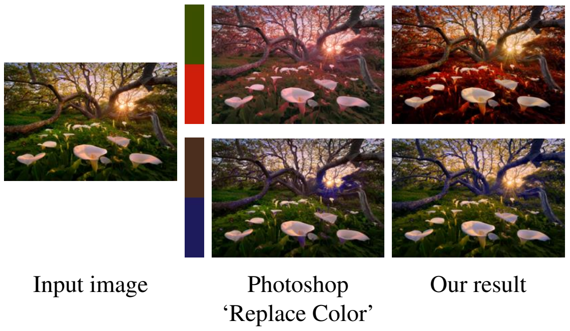


**Figure 2:** *Image recoloring comparison. In the second column, the original color is shown at the top and replacement color on the bottom for each recoloring. With Photoshop's 'Replace Color' function, the user specifies a color and 'fuzziness' value, which determines the pixels to be recolored to a target color. With layer edits, a single layer color is changed, and the change propagates through the image. Input image by Marc Adamus.*

Color replacement tools are found in popular image-editing programs. In Figure 2, we compare our image recoloring approach against Photoshop CS6. Photoshop's approach cannot handle many color blending scenarios, and fails to propagate the color changes throughout the image.

### Number of Layers

One of the free parameters in our method's automatic pipeline is the number of layers $\mathsf{N}$, which can control the granularity of an edit. In our experiments, we find that the layerings are relatively robust to the choice of $\mathsf{N}$, as long as there is enough coverage of the image color space. Figure 3 shows a recoloring example for an image and a subset of its layers under different $\mathsf{N}$. The layers corresponding to the main colors are relatively stable, and they become more specific as the number of layers increases. Increasing the number of layers also results in fewer regions outside the $[0,1]$ range, as the algorithm has to venture beyond the convex hull of the colors less often in order to correctly reconstruct the image. In this example, we can achieve similar recoloring results by changing one or two layers.

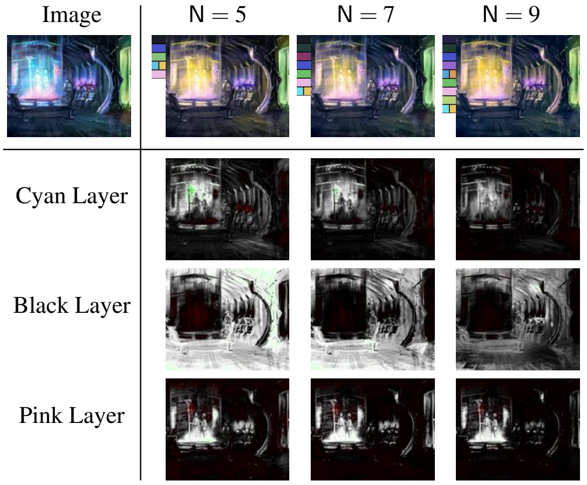


**Figure 3:** *Recoloring results as the number of layers $\mathsf{N}$ increases. Palette colors were chosen automatically. Here, we try to color the hologram light orange by changing layer colors. We can achieve this with one edit for $\mathsf{N}=5$ and $\mathsf{N}=7$, and with two edits for $\mathsf{N}=9$. The base layers are relatively consistent across different $\mathsf{N}$, and their scope decreases as the number of layers increases. Input image by Dave Revoy.*

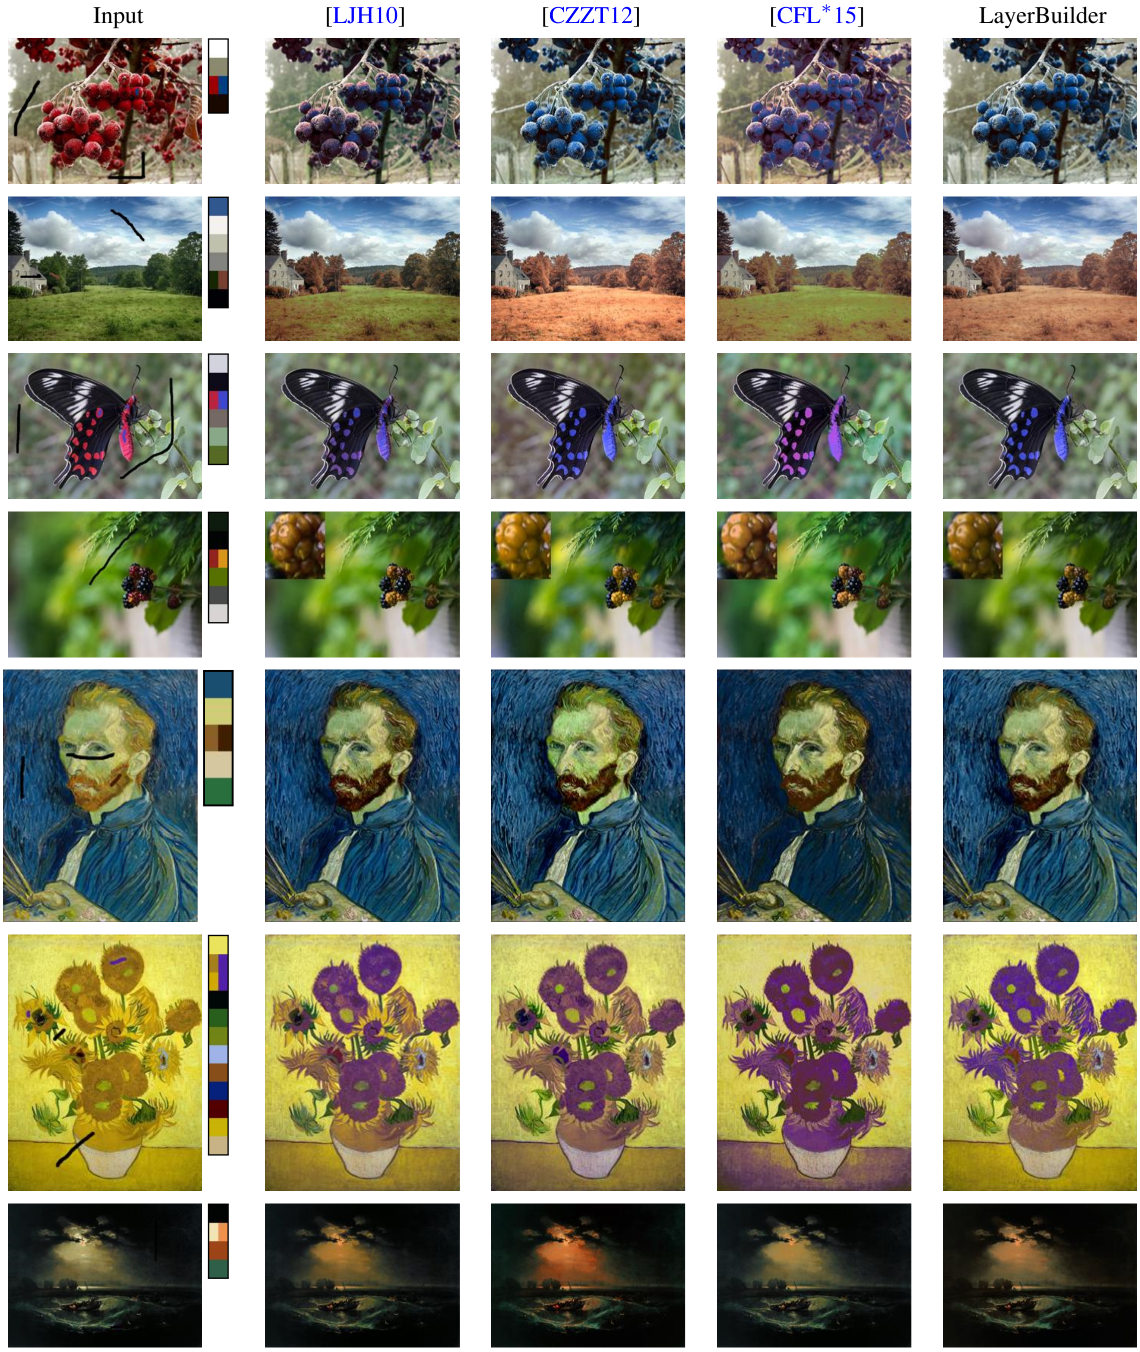


**Figure 1:** *Image recoloring comparison. The first column shows the input strokes to [LJH10] and the palette change for LayerBuilder, [CZZT12], and [CFL*15]. Colored strokes indicate a change in color on the selected pixels, while black strokes constrain the pixels to stay the same color. Colored strokes indicate a change in color on the selected pixels, while black strokes constrain the pixels to stay the same color. Similar to [CZZT12], our method often produces natural results even in the presence of challenging color blending scenarios while being faster. RBF interpolation [LJH10] and palette-based RBF interpolation [CFL*15] often produce more artifacts at color boundaries and blending regions. Input photos by Flickr users kamcmillan, arian.suresh, A Guy Taking Pictures, and ansk.*

## Appendix: Pattern Coloring Features

We adapt many of the shape features in the coloring model of Lin and colleagues [LRFH13] to work for layers. Otherwise, we use the same color properties, training process, and sampling process. Here are the shape features we considered, with novel features indicated by an asterisk:

**Relative Size** is the mean weight per pixel in that layer.

**Relative Size over Max** is the relative size of a layer divided by the maximum relative size of all layers in the image

**Radial Distance** is the Euclidean distance between the weighted centroid of the layer to the center of the image.

**Elongation** measures the width of a layer compared to its length. We use PCA on the layer weights and obtain the first and second eigenvalues $\lambda_1$ and $\lambda_2$. Elongation is then $\frac{\lambda_2}{\lambda_1}$

**Bag-of-Words*** for the layer is a histogram over a set of 50 visual words clustered from the training set of layered images. It measures how many of each word can be found in the layer. To extract visual words, we use the SIFT detector and descriptors in the OpenCV library

**Contribution Histogram*** measures the distribution in weights of the layer. It is computed as a histogram of the weights over 4 bins: $(-\infty, 0.25], (0.25, 0.5], (0.5, 0.75], (0.75, \infty)$.

**Overlap** between two layers is computed as the normalized dot product between the layer weights. To detect adjacent but not overlapping layers, we first add Gaussian blur to the layer weights. Overlap replaces Lin and colleagues' enclosure strengths.

## References

[CFL*15] CHANG H., FRIED O., LIU Y., DIVERDI S., FINKELSTEIN A.: Palette-based photo recoloring. *ACM Transactions on Graphics (Proc. SIGGRAPH) 34*, 4 (July 2015). 2

[CZZT12] CHEN X., ZOU D., ZHAO Q., TAN P.: Manifold preserving edit propagation. *ACM Transactions on Graphics (TOG) 31*, 6 (2012), 132. 2

[LJH10] LI Y., JU T., HU S.-M.: Instant propagation of sparse edits on images and videos. In *Computer Graphics Forum* (2010), vol. 29, pp. 2049–2054. 2

[LRFH13] LIN S., RITCHIE D., FISHER M., HANRAHAN P.: Probabilistic color-by-numbers: Suggesting pattern colorizations using factor graphs. In *ACM SIGGRAPH 2013 papers* (2013), SIGGRAPH '13. 3
